# Supplementary material for: Information Theoretic Measures of Causal Influences during Transient Neural Events
Source: arXiv:2209.07508 source file (2022-09-15)
Supplement: Supplementary file 1 [file supplementaryMaterial.tex]

\documentclass{article}

\usepackage[a4paper, total={7in, 9in}]{geometry}

\usepackage[utf8]{inputenc} % allow utf-8 input
\usepackage[T1]{fontenc}    % use 8-bit T1 fonts
\usepackage{hyperref}       % hyperlinks
\usepackage{url}            % simple URL typesetting
\usepackage{booktabs}       % professional-quality tables
\usepackage{amsfonts}       % blackboard math symbols
\usepackage{nicefrac}       % compact symbols for 1/2, etc.
%\usepackage{microtype}      % microtypography
\usepackage{lipsum}		% Can be removed after putting your text content
\usepackage{graphicx}
\usepackage{natbib}
\usepackage{doi}
\usepackage{color}
\usepackage{amsmath}
\usepackage{mathtools}

\makeatletter
\@addtoreset{subfigure}{figure}
\makeatother
%\setcitestyle{square} % for Physics and Applied Mathematics and Statistics articles
\usepackage{xr-hyper}
\usepackage{url,hyperref,lineno,subcaption,float,graphicx,fontenc}
\usepackage[onehalfspacing]{setspace}

\newcommand{\michel}[1]{{\small [\textcolor{red}{{\bfseries Michel}: #1}]}}
\newcommand{\Kaidi}[1]{{\small [\textcolor{blue}{{\bfseries Kaidi}: #1}]}}
\newcommand{\Revised}[1]{{\small [\textcolor{teal}{{\bfseries}#1}]}}

%used for \coloneqq
\usepackage{mathtools}
\usepackage{standalone}
%used for figure 1
\usepackage{tikz}
\usepackage{tkz-graph}
\usetikzlibrary{shapes,positioning}
\usetikzlibrary{arrows.meta}
\usetikzlibrary{matrix}
\usetikzlibrary{calc}

% define indepedent symbol
\newcommand\indep{\protect\mathpalette{\protect\independenT}{\perp}}
\def\independenT#1#2{\mathrel{\rlap{$#1#2$}\mkern2mu{#1#2}}}
\usepackage{comment}
\specialcomment{comnt}{\color{gray}}{\color{black}}
\excludecomment{comnt}

\newtheorem{defn}{Definition}
\newtheorem{expl}{Example}
\newtheorem{prop}{Proposition}
\newtheorem{thm}{Theorem}

\setcounter{equation}{0}
\setcounter{figure}{0}
\setcounter{table}{0}
\setcounter{page}{1}
\renewcommand{\theequation}{S\arabic{equation}}
\renewcommand{\thefigure}{S\arabic{figure}}
\renewcommand{\bibnumfmt}[1]{[S#1]}
\renewcommand{\citenumfont}[1]{S#1}
% Leave a blank line between paragraphs instead of using \\

%	\firstpage{1}

\def\helvetica{\fontfamily{phv}\selectfont}
\def\helveticaitalic{\fontfamily{phv}\itshape\selectfont}
\def\helveticabold{\fontfamily{phv}\bfseries\selectfont}
\def\helveticabolditalic{\fontfamily{phv}\bfseries\itshape\selectfont}

\title{Supplementary Materials}

\begin{document}
%	\onecolumn

\maketitle
\appendix


%\begin{center}
%	\textbf{\large Supplementary Materials}\\[.2cm]
%\end{center}




\section{Structural causal models} \label{app:SCM}
We introduce first important tools to address questions pertaining to causality. Interestingly, these tools apply to probabilistic models that do not necessary include time information. This framework relies on structural equations of the form
\[
Y \coloneqq f(X_1,\,\cdots,\,X_k,\,\epsilon)
\]
where the right hand side determines the assignment of values on the left-hand side. In the most usual case, $Y$ and $\{X_j\}_{j \in \{1, \cdots, k\}}$ represent observed variables and $\epsilon$ a variable accounting for (unobserved) exogenous effects. Combining structural equations allows building Structural Causal Models (SCM) that describes dependencies between multiple observed variables.
\begin{defn}[Structural Causal Model (SCM) (see e.g. \citep{causality_book})]\label{def:SCM}
	A $d$-dimensional structural causal model is a triplet $(\mathbb{S},P_N,\mathcal{G})$ consisting of:
	\begin{itemize}
		\item a directed acyclic graph $\mathcal{G}$ with $d$ vertices
		\item a set $\mathbb{S}$ of structural equations 
		\[
		V_j \coloneqq f_j(\textbf{PA}_j,N_j), j=1,\dots,d,
		\]
		where $\textbf{PA}_j$ are the variables indexed by the set of parents of vertex $j$ in $\mathcal{G}$
		\item a joint distribution $P_N$ over the exogenous variables $N_j$, which are assumed jointly independent.
	\end{itemize} 
\end{defn}


\begin{expl}
	Take the following linear SCM
	\begin{subequations}
		\begin{alignat}{3}
		X &\coloneqq N_1,\, N_1\sim \mathcal{N}(0,1),\\
		Z &\coloneqq N_2,\, N_2\sim \mathcal{N}(0,1),\\
		Y &\coloneqq X+Z+N_3,\, N_3\sim \mathcal{N}(0,1),\label{eq:Y_SCMexple}\\
		W &\coloneqq 2Y+N_4,\, N_4\sim\mathcal{N}(0,1),
		\end{alignat}
	\end{subequations}
	with the associated graph represented in Figure~\ref{fig:biasSCM}A. 
\end{expl}

One attractive feature of this formalism is that an SCM's graphical representation entails important properties of the underlying distribution of variables $\{V_k\}$ (see e.g. \citep{Bishop:2006:PRM:1162264}).

\begin{prop}[Markov properties] For a given SCM $(\mathbb{S},P_N,\mathcal{G})$, the joint distribution $P_V$ is Markovian with respect to $\mathcal{G}$, i.e. it satisfies the following properties:
	\begin{enumerate}
		\item (local Markov property) each variable $V_j$ is independent of its non-descendants given its parents $\textbf{PA}_j$,
		\item (Markov factorization property) assume the joint distribution $P_V$ has a density, then
		\[
		p(\textbf{v}) = p(v_1,\dots,v_d) = \prod_{j=1}^d p(v_j|\textbf{pa}_j) 
		\]
	\end{enumerate}
	
\end{prop}

\begin{figure}[H] 
	\centering
	\includegraphics[width=.3\textwidth]{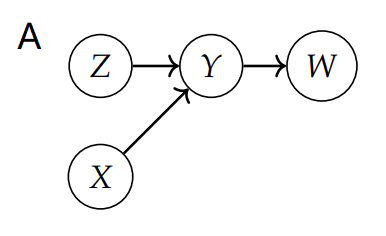}
	\caption{(A) Example of graphical representations of structural causal models. (B) Graphical representation including a sampling node, indicating that sample selection is a function of $X$ only.}
\end{figure} \label{fig:biasSCM}

These two properties are rather intuitive consequences of the definition of structural equations. As an example, the graphical model represented in Figure~\ref{fig:biasSCM}A entails that $P(X,Y,Z,W)=P(W|Y)P(Y|X,Z)P(Z)P(X)$. In addition, the concept of $d$-separation allows assessing systematically the conditional independences between subsets of nodes in $\mathcal{G}$ based on graphical criteria (see e.g. \cite{pearl2000causality}).
\begin{defn}[$d$-separation]
	A path $p$ in graph $\mathcal{G}$ is said to be $d$-separated by a set of nodes $Z$ if either: (1) $p$ contains a chain $i\rightarrow m\rightarrow j$ or a fork  $i\leftarrow m\rightarrow j$ such that the middle node $m$ is in $Z$, or (2) 
	$p$  contains a collider  $i\rightarrow m\leftarrow j$ such that the middle node $m$ is not in $Z$ and such than no descendant of $m$ is in $Z$.
	
	$Z$ is said to $d$-separate $X$ from $Y$ in $\mathcal{G}$ if and only if $Z$ blocks every path from a node in $X$ to a node in $Y$. This property is denoted
	$X \indep_\mathcal{G} Y|Z$.
\end{defn}
Indeed, $d$-separation allows stating \textit{global Markov property} (see e.g. \citep{causality_book}).

\begin{prop}[Global Markov property]\label{prop:globalMarkov}
	For a given SCM $(\mathbb{S},P_N,\mathcal{G})$ and subsets of nodes $X$, $Y$, $Z$ in $\mathcal{G}$,  then
	\[
	X\indep_\mathcal{G} Y|Z  \Rightarrow X\indep_{P_V} Y|Z\,.
	\]
\end{prop}
\setcounter{expl}{0}
\begin{expl}[continued]
	The graphical model of Figure~\ref{fig:biasSCM}A implies $Z \indep X$ and $Z\indep W|Y$. Interestingly, it does not imply $Z \indep X|Y$ because of the collider $Z\rightarrow Y \leftarrow X$.	
\end{expl}
Note that $d$-separation only implies conditional independence. The reverse implication requires an additional assumption regarding the relation between the graph and the random variable called faithfulness (see for example \cite[chapter 6]{causality_book}). As an example, under the faithfulness assumption, the graphical model of Figure~\ref{fig:biasSCM}A entails that $X$ and $Z$ are dependent given $Y$. 

\subsection{Interventions}
The SCM framework allows modeling  interventions performed on a system. Classical interventions in an SCM amount to impose a fixed value to a random variable, but the framework allows a much broader class of modifications of the SCM. For instance, instead of a constant, one can do \textit{soft interventions} where we impose the value of a variable to be draw from a given distribution, independently from other variables in the SCM. In general, taking the SCM of Definition~\ref{def:SCM}, intervening on $V_k$ consists in replacing its structural assignment by a new one:
\[
V_k\coloneqq \widetilde{f_k}(\widetilde{\textbf{PA}_k},\widetilde{N_k})\,.
\] 
The resulting modified distribution $\widetilde{P}_V=P_V^{\text{ do}(V_k\coloneqq\widetilde{f_k}(\widetilde{\textbf{PA}_k},\widetilde{N_k}))}$ is called intervention distribution (see e.g. \cite[chapter 6]{causality_book}).
\setcounter{expl}{0}
\begin{expl}[continued]
	In the previous SCM example of Figure~\ref{fig:biasSCM}A, $P_V^{\text{ do}(Y\coloneqq y_0)}$ is the distribution entailed by the SCM that replaces equation~(\ref{eq:Y_SCMexple}) by the new structural assignment: $Y\coloneqq y_0$, and keeps all other structural equations. We can see from the causal graph that the marginal distributions of $X$ and $Z$ will not be affected by this interventions, contrary to $W$.
\end{expl}

\section{Proof of insensitivity of DCS to deterministic perturbations} \label{app:insensit_dcs}
Similar to the derivation for TE in the main text, we have
\begin{multline*}% \label{eq: TE definition}
	\text{DCS}(\widetilde{X}^2_t\rightarrow \widetilde{X}^1_t) 
	= \int 
	\widetilde{p}(X^1_t,\boldsymbol{X}^1_{p,t},\boldsymbol{X}^2_{p,t}) 
	\log 
	\frac{\widetilde{p}(X^1_t|\boldsymbol{X}^1_{p,t}, \boldsymbol{X}^2_{p,t})}{ \int \widetilde{p}(X^1_t|\boldsymbol{X}^1_{p,t},{\boldsymbol{X}^2_{p,t}})\widetilde{p}({\boldsymbol{X}^2_{p,t}})
		\mathrm{d}{\boldsymbol{X}^2_{p,t}}
		%\widetilde{p}(X^1_t|\boldsymbol{X}^1_{p,t})
	}\, \mathrm{d} X^1_t \mathrm{d} \boldsymbol{X}^1_{p,t} \mathrm{d} \boldsymbol{X}^2_{p,t}\\
	= \int {p}(X^1_t\!-\!U_t,\boldsymbol{X}^1_{p,t}\!-\!\mathbf{U}_{p,t},\boldsymbol{X}^2_{p,t}\!-\!\mathbf{V}_{p,t}) 
	\log\!\! 
	\frac{{p}(X^1_t\!-\!U_t|\boldsymbol{X}^1_{p,t}\!-\!\mathbf{U}_{p,t}, \boldsymbol{X}^2_{p,t}\!-\!\mathbf{V}_{p,t})}
	{\int p(X^1_t-U_t|\boldsymbol{X}^1_{p,t}-\mathbf{U}_{p,t},{\boldsymbol{X}^2_{p,t}-\mathbf{V}_{p,t}})p({\boldsymbol{X}^2_{p,t}-\mathbf{V}_{p,t}})
		\mathrm{d}{\boldsymbol{X}^2_{p,t}}}\\
	\mathrm{d} X^1_t \mathrm{d} \boldsymbol{X}^1_{p,t} \mathrm{d}\boldsymbol{X}^2_{p,t}\\
	= \int{p}(X^1_t,\boldsymbol{X}^1_{p,t},\boldsymbol{X}^2_{p,t}) 
	\log 
	\frac{{p}(X^1_t|\boldsymbol{X}^1_{p,t},\boldsymbol{X}^2_{p,t})}
	{\int p(X^1_t|\boldsymbol{X}^1_{p,t},{\boldsymbol{X}^2_{p,t}})p({\boldsymbol{X}^2_{p,t}})
		\mathrm{d}{\boldsymbol{X}^2_{p,t}}}
	\, \mathrm{d} X^1_t \mathrm{d} \boldsymbol{X}^1_{p,t} \mathrm{d} \boldsymbol{X}^2_{p,t}\\
	= \text{DCS}({X^2_t}\rightarrow {X^1_t})\,.
\end{multline*}


\section{Selection bias} \label{app:bias}
The SCM approach allows us to draw conclusions about statistical and causal inference procedures based only on the graphical representation. One interesting question that has been addressed in such a way is selection bias \citep{bareinboim2014recovering,bareinboim2012controlling}. Selection bias points to the practical issue of how selection of data points affect the inference of relevant quantities in a statistical or causal model \citep{hernan2004structural,horwitz1978alternative}. To address this question, one can consider a binary random variable $S$ that takes the value 1 when a data point is selected and zero otherwise. It is frequently the case that $S$ depends (causally) on other variables of the SCM under consideration and as such it can be included as a special node in the graphical representation, as exemplified in Figure~\ref{fig:biasSCM}. Given the original distribution $P$ over the variables, sample selection generally results in a different distribution $P_S$. 

\subsection{Recoverability with Sampling Selection Bias} \label{app:bias_theory}




In the simplest two-node SCM, the identifiability or recoverability of the effect based on different sampling methods has been investigated in \citep{bareinboim2014recovering}. 

\begin{figure}
	\centering
	\includegraphics[width=.6\textwidth]{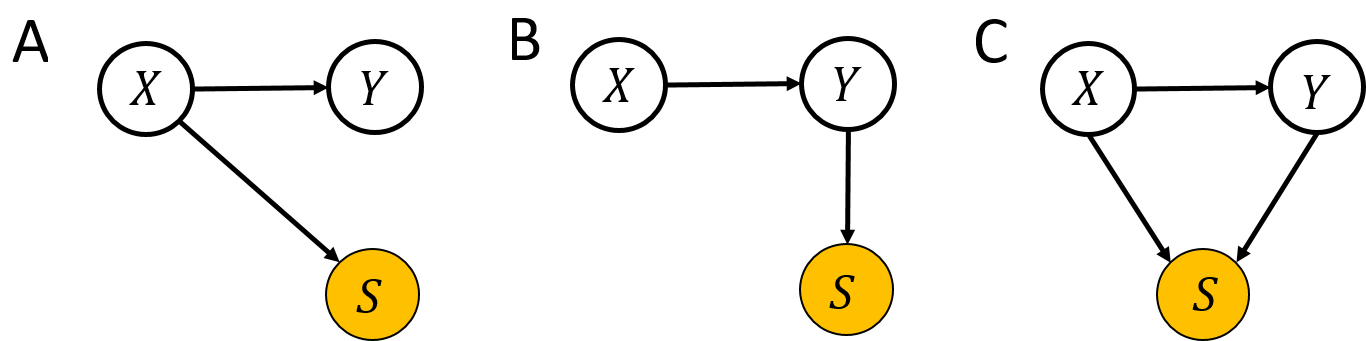}
	\caption{SCM, selection bias and recoverability (adapted from \cite{bareinboim2014recovering}).
		(A) SCM describing sample selection based on $X$, leading to identifiability of $P(Y|X)$ based on selected data. 
		(B) SCM describing sample selection based on $Y$, leading to non-identifiability of $P(Y|X)$ based on selected data. 
		(C) SCM describing sample selection based on both $X$ and $Y$, leading to non-identifiability of $P(Y|X)$ based on selected data.	
		\label{fig:scm_bias}}
	
\end{figure}


Figure~\ref{fig:scm_bias}A, B, C show three sampling conditions in a two-node SCM consisting of variables $X$ and $Y$ (with $X$ causing $Y$). 
Sampling is represented by binary variable $S$ in an additional node designed as descendant for either $X$ or $Y$.
$S$ takes the value 1 when a data point is selected and zero otherwise.
In  Figure~\ref{fig:scm_bias}A, sample selection is a function of $X$ only, while Figure~\ref{fig:scm_bias}B describes a sample selection based on $Y$ only.
Figure~\ref{fig:scm_bias}C presents the condition where sample selection depends on both variables.


In this model, we are interested in estimating the conditional propability of $P(Y|X)$ from sampled data.
What is critical is whether $P(Y|X)$ can be recovered from the joint distribution  of the selected samples $(X,Y)|S=1$ given different sampling scenarios. \citet{bareinboim2014recovering} show that, under standard assumptions, a necessary and sufficient condition for recoverability is conditional independence between target variable $Y$ and selection variable $S$, given conditioning variable $X$ ($Y\indep S|X)$) such that $P(Y|X,S=1)=P(Y|X)$. 
For the scenarios of Figure~\ref{fig:scm_bias}, this implies that $P(Y|X)$ can be recovered $(X,Y)|S=1$ in the case of Figure~\ref{fig:scm_bias}A, but not in  Figure~\ref{fig:scm_bias}B and Figure~\ref{fig:scm_bias}C. 

The rationale is simple according to the $d$-separation rules (see Section~\ref{app:SCM} for details). 
In the condition of Figure~\ref{fig:scm_bias}A, conditioning on $X$ corresponds to the ``fork'' case in the $d$-separation rules, indicating that the conditional independence $Y\indep S|X$ is satisfied. 
On the contrary, Figure~\ref{fig:scm_bias}B shows the condition where such that $P(Y|X)$ is not recoverable from sample selected data because the above conditional independence requirement ($Y$ independent of $S$ given $X$) is not satisfied. 
For Figure~\ref{fig:scm_bias}B, detailed proof has been provided in \citet{bareinboim2014recovering}.
%, which is included in the appendix.\design{decide whether to include in the appendix..}
The case in Figure~\ref{fig:scm_bias}C corresponds to the ``collider'' case of $d$-separation where a common observed descendant induces extra dependency between the ancestors.



\subsection{Recoverability with Sampling Selection Bias in VAR($p$) models} \label{app:bias_VAR}

Applying the aforementioned relationships between $X$, $Y$ and $S$ to VAR models, we can easily access the recoverabilities of conditionals in the SCMs, thus knowing whether the causal arrows can be estimated.

For example, in the SCM in Figure 3A of the main text, $\boldsymbol{X}^2_{p,t}$ $d$-separates $S$ and  $X^1_{t}$ for every negative $t^{\prime}$, thus $P(X^1_t \mid \boldsymbol{X}^1_t, \boldsymbol{X}^2_t)$ is recoverable such that:
\[
P\left(X_{t}^{1} \mid\boldsymbol{X}^1_{p,t}, \boldsymbol{X}^2_{p,t}, S\right) =P\left(X_{t}^{1} \mid \boldsymbol{X}^1_{p,t}, \boldsymbol{X}^2_{p,t}\right)
\] 
This is also true for positive $t^{\prime}$ as $S$ is dependent on the indirect cause of the causal arrows. 
For the non-causal direction, the selection node as $S$ is similar to Figure~\ref{fig:scm_bias}C such that for negative $t^{\prime}$ there is
\[
P\left(X_{t}^{2} \mid \boldsymbol{X}^1_{p,t}, \boldsymbol{X}^2_{p,t}, S\right) 
\neq P\left(X_{t}^{2} \mid \boldsymbol{X}^1_{p,t}, \boldsymbol{X}^2_{p,t}\right) 
= P\left(X_{t}^{2} \mid  \boldsymbol{X}^2_{p,t}\right)
\] 
For positive $t^{\prime}$, $S$ only depends on the indirect cause for all arrows such that
\[
P\left(X_{t}^{2} \mid \boldsymbol{X}^1_{p,t}, \boldsymbol{X}^2_{p,t}, S\right) 
= P\left(X_{t}^{2} \mid \boldsymbol{X}^1_{p,t}, \boldsymbol{X}^2_{p,t}\right) 
= P\left(X_{t}^{2} \mid  \boldsymbol{X}^2_{p,t}\right)
\] 
The reasoning is similar for Figure~\ref{fig:scm_var5}A, which represents filtering the original signal and detect events with template matching approaches. For Figure 3B and Figure~\ref{fig:scm_var5}B, $S$ can never be understood as purely dependent on the cause for negative $t^{\prime}$. For example, for the causal arrow in $P\left(X_{t-1}^{2} \mid \boldsymbol{X}^1_{p,t-2}, \boldsymbol{X}^2_{p,t-2}, S\right)$, $\boldsymbol{X}^1_{p,t-2}$ does not $d$-separates $S$ and  $\boldsymbol{X}_{t-1}^{2}$ due to the causal arrow from  $\boldsymbol{X}_{t-1}^{2}$ to $X_{t}^{1}$. Thus none of the conditionals can be recoverable for negative $t^{\prime}$, but the opposite for positive $t^{\prime}$.


\begin{figure}
	\centering
	\includegraphics[width=\textwidth]{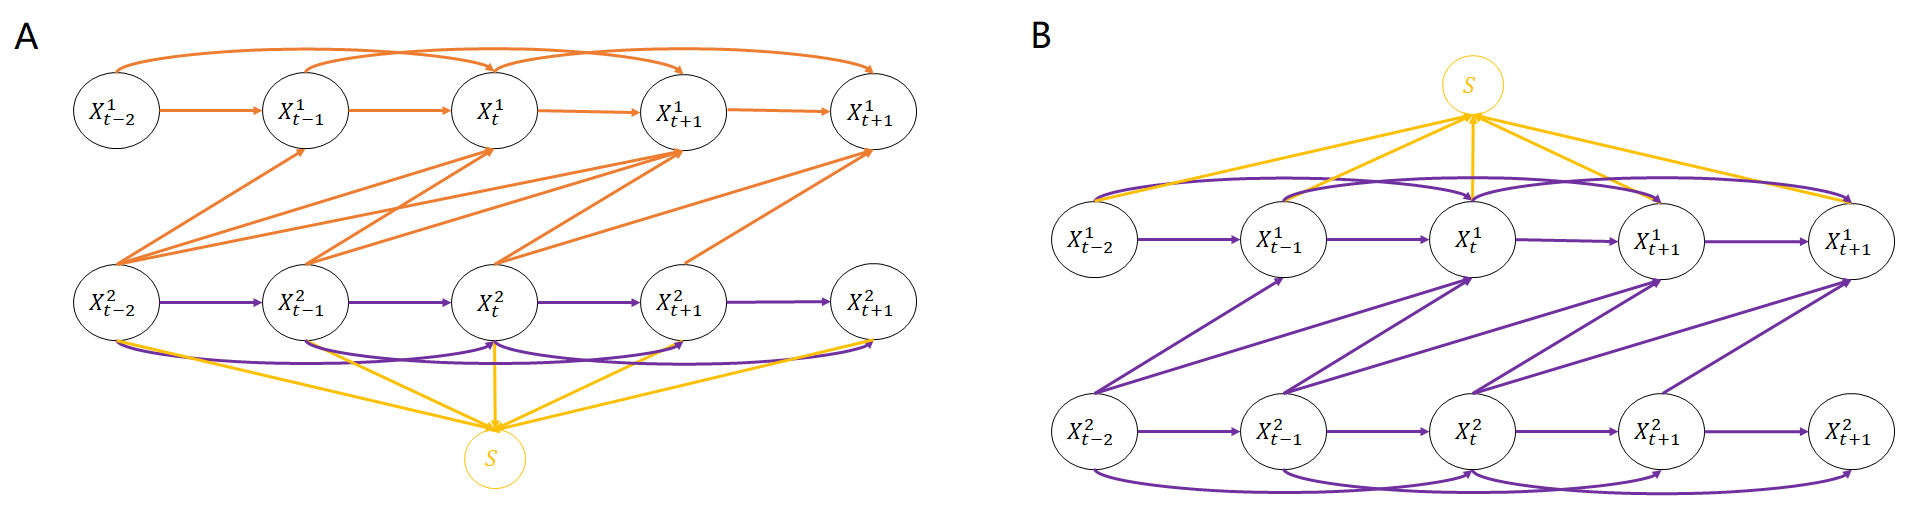}
	\caption{
		(A) SCM of a bi-variate VAR(2) model with uni-directional coupling from $X^2$ to $X^1$ and a selection node S depending on states of the cause variable before peri-event time ($t^{\prime}<=0$). The selection node S represents partial selection of samples due to thresholding of the detection signal obtained with template matching with the original signal. Orange arrows makes the recoverable arrows with the current selection node, while purple arrows indicates the unrecoverable ones.  
		(B) The same SCM as in (A) with the selection node depending in a similar way on the effect signal.	
		\label{fig:scm_var5}}
	
\end{figure}


\section{Derivations for time-varying causality measures}

\subsection{Time-varying VAR($p$) model}
Following the introduction, the candidate measures include Granger causality (GC), Tranfer Entropy (TE) and Causal Strength (CS) \citep{janzing_2013}, where we extend them into a time-varying version to address the non-stationarity of transient events.
In addition to their potential information theoretic formulations, the measures will also be formulated in a time-varying bivariate system consisting two variables $X^1$ and $X^2$. 
%\marginpar{The notations are designed to be consistent with the VAR model for peri-event snapshots, as introduced in Section~\ref{sec:var_estim}} 
The system is assumed as a inhomogeneous bivariate $p$-ordered Vector Autoregressive (VAR($p$)) model.
At each time $t$, the current state $\boldsymbol{X}_t = [X^1_t, X^2_t]^\top$ is a linear function of the past (lagged) $p$ states gathered in the vector
\begin{equation}\label{eq:historyvec}
	\boldsymbol{X}_{p,t} = [{\boldsymbol{X}^1_{p,t}}^\top, {\boldsymbol{X}^2_{p,t}}^\top]^\top = [X^1_{t-1}, X^1_{t-2}, ..., X^1_{t-p}, X^2_{t-1}, X^2_{t-2}, ..., X^2_{t-p}]^\top
\end{equation}
and the exogeneous inputs as the innovation term
\[
\boldsymbol{\eta}_t = [\eta_t^1, \eta_t^2]^\top
\]
in the following form
\begin{equation} \label{eq:var_inhomo_ch4}
	\boldsymbol{X}_t \coloneqq A_t \boldsymbol{X}_{p,t}+\boldsymbol{\eta}_t\,,\boldsymbol{\eta}_t\sim \mathcal{N}(\mathbf{k}_t,\Sigma_t)\,,
\end{equation}
where the autoregressive coefficient $A_t = \begin{bmatrix}
	\mathbf{a}_t^\top & \mathbf{b}_t^\top\\
	\mathbf{c}_t^\top & \mathbf{d}_t^\top
\end{bmatrix}$, the innovation mean
$k = \begin{bmatrix}
	k_t^1 \\
	k_t^2
\end{bmatrix}$,
and innovation covariance $\Sigma_t= \begin{bmatrix}
	\sigma_{1,t} & 0\\
	0 & \sigma_{2,t}
\end{bmatrix}$ are the model parameters.
The column sign suggests that the VAR model can be interpreted as a data generation mechanism, which is critical to the SCM framework (Section~\ref{app:SCM}).
Elements of the coefficient matrix $\mathbf{a}_t$,$\mathbf{b}_t$,$\mathbf{c}_t$ and $\mathbf{d}_t$ are all $p$-dimensional vectors. Expanding the vector version of Eq.~\ref{eq:var_inhomo_ch4} using Eq.~\ref{eq:historyvec}, the equation can be rewritten as:
\begin{equation} \label{eq:full_model_x1_inhomo}
	X^1_t = \mathbf{a}^{\top}_t \boldsymbol{X}^1_{p,t} + \mathbf{b}^{\top}_t \boldsymbol{X}^2_{p,t} +\eta^1_t\,,\quad\eta^1_t \sim \mathcal{N}(k^1_t,\,\sigma_{1,t})\,.
\end{equation}
\begin{equation} \label{eq:full_model_x2_inhomo}
	X^2_t = \mathbf{c}^{\top}_t \boldsymbol{X}^1_{p,t} + \mathbf{d}^{\top}_t \boldsymbol{X}^2_{p,t} +\eta^2_t\,,\quad\eta^2_t \sim \mathcal{N}(k^2_t,\,\sigma_{2,t})\,,
\end{equation}

\subsection{Derivation of KL-divergence between two uni-variate Gaussians} \label{app:KL_gaussian}

Time-varying TE, DCS and rDCS are formulated as the KL divergence between the corresponding actual and counterfactual conditions. Thus we first present the KL divergence between two uni-variate Gaussian variables. 

We denote the gaussian for the actual condition as $p(x) = \mathcal{N}(\mu_a, \sigma^2_a)$, and the counterfactual gaussian as $q(x) = \mathcal{N}(\mu_c, \sigma^2_c)$. 
Then the KL divergence between $p(x)$ and $q(x)$ is 

\[
\begin{aligned} D_{KL}(p||q) 
	&= - \int p(x) \log q(x) dx + \int p(x) \log p(x) dx\\\\ 
	&=\int \left[\log( p(x)) - log( q(x)) \right] p(x) dx\\\\ 
	&=\int \left[ -\frac{1}{2} \log(2\pi) - \log(\sigma_a) - \frac{1}{2} \left(\frac{x-\mu_a}{\sigma_a}\right)^2 + \frac{1}{2}\log(2\pi) + \log(\sigma_c) + \frac{1}{2} \left(\frac{x-\mu_c}{\sigma_c}\right)^2 \right]\times \\\\ &\frac{1}{\sqrt{2\pi}\sigma_a}\exp\left[-\frac{1}{2}\left(\frac{x-\mu_a}{\sigma_a}\right)^2\right] dx\\\\ 
	&=\int \left\{\log\frac{\sigma_c}{\sigma_a} + \frac{1}{2} \left[ \left(\frac{x-\mu_c}{\sigma_c}\right)^2 - \left(\frac{x-\mu_a}{\sigma_a}\right)^2 \right] \right\}\times \frac{1}{\sqrt{2\pi}\sigma_a} \exp\left[-\frac{1}{2}\left(\frac{x-\mu_a}{\sigma_a}\right)^2\right] dx\\\\ 
	&=\mathbb{E}_{p} \left[\log\frac{\sigma_c}{\sigma_a} + \frac{1}{2} \left[ \left(\frac{x-\mu_c}{\sigma_c}\right)^2 - \left(\frac{x-\mu_a}{\sigma_a}\right)^2 \right]\right]\\\\ 
	&=\log\frac{\sigma_c}{\sigma_a} + \frac{1}{2\sigma_c^2} \mathbb{E}_{p} \left[(X-\mu_c)^2\right] - \frac{1}{2\sigma_a^2} \mathbb{E}_{p} \left[(X-\mu_a)^2\right]\\\\ 
	&=\log\frac{\sigma_c}{\sigma_a} + \frac{1}{2\sigma_c^2} \mathbb{E}_{p} \left[(X-\mu_c)^2\right] - \frac{1}{2}
\end{aligned} 
\]

Note that 
\[
\begin{aligned} (X - \mu_c)^2 
	&= (X-\mu_a+\mu_a-\mu_c)^2 \\\\ 
	&= (X-\mu_a)^2 + 2(X-\mu_a)(\mu_a-\mu_c) + (\mu_a-\mu_c)^2
\end{aligned} 
\]

Therefore,
\begin{multline} \label{eq:app_KL}
	D_{KL}(\mathcal{N}(\mu_a,\,\sigma^2_a)||\mathcal{N}(\mu_c,\,\sigma^2_c))
	=\log\frac{\sigma_c}{\sigma_a} + \frac{1}{2\sigma_c^2} \mathbb{E}_{p}\left[(X-\mu_a)^2\right] \\
	+ 2(\mu_a-\mu_c)\mathbb{E}_{p}\left[X-\mu_a\right] + (\mu_a-\mu_c)^2 - \frac{1}{2}\\ 
	=\frac{1}{2}\log\frac{\sigma^2_c}{\sigma^2_a} + \frac{\sigma_a^2 + (\mu_a-\mu_c)^2}{2\sigma_c^2} - \frac{1}{2}
\end{multline}

\subsection{Conditional mean and variance for the actual condition}

The actual condition defined for TE, DCS and rDCS is that the current state of $X^1_t$ is dependent on the past of both $X^1$ and $X^2$, denoted as
\[
\mathcal{N}(\mu_a,\sigma_a^2) = p(X^1_t|\boldsymbol{X}^1_{p,t},\boldsymbol{X}^2_{p,t})\,.
\]
The dynamics of $X^1_t$ is described by the structural equation
\begin{equation}\label{eq:app_actual_VAR}
	X^1_t = \mathbf{a}^{\top}_t \boldsymbol{X}^1_{p,t} + \mathbf{b}^{\top}_t \boldsymbol{X}^2_{p,t} +\eta^1_t\,,\quad\eta^1_t \sim \mathcal{N}(k^1_t,\,\sigma_{1,t})\,.
\end{equation}


Therefore, the time-varying conditional mean and variance can be derived as
\[
\mu_a = \mathbb{E}[\mathbf{a}_t^\top \boldsymbol{X}^1_{p,t}+\mathbf{b}_t^\top \boldsymbol{X}^2_{p,t}+\eta^1_t|\boldsymbol{X}^1_{p,t},\boldsymbol{X}^2_{p,t}] = \mathbf{a}_t^\top \boldsymbol{X}^1_{p,t}+\mathbf{b}_t^\top \boldsymbol{X}^2_{p,t}+k^1_t
\]
\[
\sigma_a^2 = \operatorname{Var}[\mathbf{a}^\top \boldsymbol{X}^1_{p,t}+\mathbf{b}^\top \boldsymbol{X}^2_{p,t}+\eta^1_t|\boldsymbol{X}^1_{p,t},\boldsymbol{X}^2_{p,t}] = \operatorname{Var}[\eta^1_t|\boldsymbol{X}^1_{p,t},\boldsymbol{X}^2_{p,t}] =  \sigma_{1,t} 
\]
\subsection{Transfer Entropy} \label{app:TE}
For TE, as the conditional probability representing the "counterfactual" condition takes the form
\[
\mathcal{N}(\mu_c,\sigma_c^2) = p(X^1_t|\boldsymbol{X}^1_{p,t})\,.
\]
Resulting from the same model in Eq.~\ref{eq:app_actual_VAR}, the mean and variance can be derived as
\begin{equation*}
	\mu_c = \mathbb{E}[\mathbf{a}_t^\top \boldsymbol{X}^1_{p,t}+\mathbf{b}_t^\top \boldsymbol{X}^2_{p,t}+\eta^1_t|\boldsymbol{X}^1_{p,t}] 
	= \mathbf{a}_t^\top \boldsymbol{X}^1_{p,t}|\boldsymbol{X}^1_{p,t}+\mathbf{b}_t^\top \mathbb{E}[ \boldsymbol{X}^2_{p,t}|\boldsymbol{X}^1_{p,t}]+k^1_t
\end{equation*}
\begin{equation*}
	\sigma_c^2 
	= \operatorname{Var}[\mathbf{a}^\top \boldsymbol{X}^1_{p,t}+\mathbf{b}^\top \boldsymbol{X}^2_{p,t}+\eta^1_t|\boldsymbol{X}^1_{p,t}]
	= \mathbf{b}_t^\top \text{Cov}[\boldsymbol{X}^2_{p,t}|\boldsymbol{X}^1_{p,t}]\mathbf{b}_t +\sigma_{1, t}
\end{equation*}
while
\begin{multline*}
	\mathbb{E}_{(\boldsymbol{X}^1_{p,t},\boldsymbol{X}^2_{p,t})}[(\mu_a-\mu_c)^2] = \mathbb{E}_{(\boldsymbol{X}^1_{p,t},\boldsymbol{X}^2_{p,t})}[(\mathbf{b}_t^\top (\boldsymbol{X}^2_{p,t} - \mathbb{E}[\boldsymbol{X}^2_{p,t}|\boldsymbol{X}^1_{p,t}]))^2] \\
	= \mathbf{b}_t^\top \mathbb{E}[(\boldsymbol{X}^2_{p,t}-\mathbb{E}|\boldsymbol{X}^2_{p,t}])(\boldsymbol{X}^2_{p,t}-\mathbb{E}|\boldsymbol{X}^2_{p,t}|\boldsymbol{X}^1_{p,t}])^\top] \mathbf{b}_t = \mathbf{b}_t^\top \operatorname{Cov}[\boldsymbol{X}^2_{p,t}|\boldsymbol{X}^1_{p,t}]] \mathbf{b}_t
\end{multline*}
Plugging the expressions of $\mu_a$, $\mu_c$, $\sigma^2_a$ and $\sigma^2_c$ into Eq.~\ref{eq:app_KL}, the KL divergence can be derived as
\[
	\text{TE}(X^2_t\rightarrow X^1_t)  = D_{KL}(\mathcal{N}(\mu_a,\,\sigma^2_a)||\mathcal{N}(\mu_c,\,\sigma^2_c)) =
\frac{1}{2}\log \frac{\mathbf{b}_t^\top \text{Cov}[\boldsymbol{X}^2_{p,t}|\boldsymbol{X}^1_{p,t}]\mathbf{b}_t +\sigma_{1, t}}{\sigma_{1, t}}
\]
As $\boldsymbol{X}^1_{p,t}$ and $\boldsymbol{X}^2_{p,t}$ are jointly Gaussian, the conditional variance takes the form
\[
\text{Cov}[\boldsymbol{X}^2_{p,t}|\boldsymbol{X}^1_{p,t}] = \Sigma_{\boldsymbol{X}^2_p} - \Sigma_{\boldsymbol{X}^1_p \boldsymbol{X}^2_p} \Sigma_{\boldsymbol{X}^1_p}^{-1} \Sigma_{\boldsymbol{X}^2_p \boldsymbol{X}^1_p}\,.
\]

Therefore, the expression of time-varying TE should be
\begin{equation} \label{eq:TE_inhomo_var}
	\text{TE}(X^2_t\rightarrow X^1_t) =  \frac{1}{2}\log 
	\frac{\sigma_{1, t} + \mathbf{b}_t^\top\Sigma_{\boldsymbol{X}^2_p} \mathbf{b}_t
		- \mathbf{b}_t^\top\Sigma_{\boldsymbol{X}^1_p \boldsymbol{X}^2_p} \Sigma_{\boldsymbol{X}^1_p}^{-1} \Sigma_{\boldsymbol{X}^2_p \boldsymbol{X}^1_p} \mathbf{b}_t}
	{\sigma_{1, t}}
\end{equation}

\subsection{Dynamic Causal Strength} \label{app:DCS}
For DCS, the counterfactual condition is
\[
\mathcal{N}(\mu_c,\sigma_c^2) = p^{do(X^1_t \coloneqq f(\boldsymbol{X}^1_{p,t},{\boldsymbol{X}^2_{p,t}}^\prime, \eta^1_t))}(X^1_t|\boldsymbol{X}^1_{p,t},\boldsymbol{X}^2_{p,t})
\]
with $X^1_t = \mathbf{a}_t^\top \boldsymbol{X}^1_{p,t}+\mathbf{b}_t^\top {\boldsymbol{X}^2_{p,t}}^\prime+\eta^1_t$, and ${\boldsymbol{X}^2_{p,t}}^\prime$ is a random sample drawn from the distribution $p(\boldsymbol{X}^2_{p,t})$.

Then the conditional mean is:
\[
\mu_c = \mathbb{E}[\mathbf{a}_t^\top \boldsymbol{X}^1_{p,t}+\mathbf{b}_t^\top {\boldsymbol{X}^2_{p,t}}^\prime+\eta^1_t|\boldsymbol{X}^1_{p,t},\boldsymbol{X}^2_{p,t}] = \mathbf{a}_t^\top \boldsymbol{X}^1_{p,t}+\mathbf{b}_t^\top \mathbb{E}[\boldsymbol{X}^2_{p,t}]+\eta^1_t
\]

The conditional variance is:
\begin{multline*}
	\sigma_a^2 = \operatorname{Var}[\mathbf{a}^\top \boldsymbol{X}^1_{p,t}+\mathbf{b}^\top \boldsymbol{X}^2_{p,t}+\eta^1_t|\boldsymbol{X}^1_{p,t},\boldsymbol{X}^2_{p,t}] \\
	= \operatorname{Var}[\mathbf{b}^\top {\boldsymbol{X}^2_{p,t}}^\prime|\boldsymbol{X}^2_{p,t}] + \operatorname{Var}[\eta^1_t] = \mathbf{b}^\top \operatorname{Cov}[\boldsymbol{X}^2_{p,t}] \mathbf{b} + \sigma_{1,t}
\end{multline*}

with $\operatorname{Cov}[\boldsymbol{X}^2_{p,t}] = \mathbb{E}[(\boldsymbol{X}^2_{p,t}-\mathbb{E}|\boldsymbol{X}^2_{p,t}])(\boldsymbol{X}^2_{p,t}-\mathbb{E}|\boldsymbol{X}^2_{p,t}])^\top]$.

DCS defined as the KL divergence between the actual and counterfactual conditions:
\[
\text{DCS}(X^2_t\rightarrow X^1_t) =  \mathbb{E}_{(\boldsymbol{X}^1_{p,t},\boldsymbol{X}^2_{p,t})}\left[\frac{1}{2}\log \frac{\sigma_c^2}{\sigma_a^2} - \frac{1}{2} + \frac{1}{2} \cdot \frac{\sigma_a^2+(\mu_a-\mu_c)^2}{\sigma_c^2} \right]
\]
\begin{equation*}
	\text{DCS}(X^2_t\rightarrow X^1_t)  = \frac{1}{2}\log \frac{\sigma_c^2}{\sigma_a^2} - \frac{1}{2} + \frac{1}{2} \cdot \frac{\sigma_a^2+\mathbb{E}_{(\boldsymbol{X}^1_{p,t},\boldsymbol{X}^2_{p,t})}[(\mu_a-\mu_c)^2]}{\sigma_c^2}  
\end{equation*}
while
\begin{multline*}
	\mathbb{E}_{(\boldsymbol{X}^1_{p,t},\boldsymbol{X}^2_{p,t})}[(\mu_a-\mu_c)^2] = \mathbb{E}_{(\boldsymbol{X}^1_{p,t},\boldsymbol{X}^2_{p,t})}[(\mathbf{b}_t^\top (\boldsymbol{X}^2_{p,t} - \mathbb{E}[\boldsymbol{X}^2_{p,t}]))^2] \\
	= \mathbf{b}_t^\top \mathbb{E}[(\boldsymbol{X}^2_{p,t}-\mathbb{E}|\boldsymbol{X}^2_{p,t}])(\boldsymbol{X}^2_{p,t}-\mathbb{E}|\boldsymbol{X}^2_{p,t}])^\top] \mathbf{b}_t = \mathbf{b}_t^\top \operatorname{Cov}[\boldsymbol{X}^2_{p,t}] \mathbf{b}_t
\end{multline*}

Therefore the expression of DCS can be obtained by plugging-in the means and variances of the two Gaussian distributions, 
\begin{multline*}
	\text{DCS}(X^2_t\rightarrow X^1_t) =
	\frac{1}{2}\log \frac{\mathbf{b}_t^\top \operatorname{Cov}[\boldsymbol{X}^2_{p,t}] \mathbf{b}_t + \sigma_{1,t}}{ \sigma_{1,t}} - \frac{1}{2}\\ +  \frac{1}{2} \cdot \frac{\sigma_{1,t} +\mathbf{b}_t^\top \operatorname{Cov}[\boldsymbol{X}^2_{p,t}] \mathbf{b}_t }{\mathbf{b}_t^\top \operatorname{Cov}[\boldsymbol{X}^2_{p,t}] \mathbf{b}_t + \sigma_{1,t}} 
	= \frac{1}{2}\log \frac{\mathbf{b}_t^\top \operatorname{Cov}[\boldsymbol{X}^2_{p,t}] \mathbf{b}_t + \sigma_{1,t}}{ \sigma_{1,t}}
\end{multline*}


\subsection{Relative Dynamic Causal Strength} \label{app:rDCS}

The relative Causal Strength is 'relative' in the sense that the intervention involves an independent copy of a baseline state $\boldsymbol{X}^2_{p, t_\mathit{ref}}$, instead of the lagged state ${\boldsymbol{X}^2_{p,t}}^\prime$, such that ${X^1_t}^\prime = \mathbf{a}_t^\top \boldsymbol{X}^1_{p,t}+\mathbf{b}_t^\top \boldsymbol{X}^2_{p, t_\mathit{ref}}+\eta^1_t$ for the counterfactual condition.
\[
\mathcal{N}(\mu_c,\sigma_c^2)=p^{do(X^1_t \coloneqq f(\boldsymbol{X}^1_{p,t},\boldsymbol{X}^2_{p, t_\mathit{ref}}, \eta^1_t))}(X^1_t|\boldsymbol{X}^1_{p,t},\boldsymbol{X}^2_{p,t})
\]

The conditional mean and variance for the counterfactual condition should be revised as:
\[
\mu_c = \mathbb{E}[\mathbf{a}_t^\top \boldsymbol{X}^1_{p,t}+\mathbf{b}_t^\top \boldsymbol{X}^2_{p, t_\mathit{ref}}+\eta^1_t|\boldsymbol{X}^1_{p,t},\boldsymbol{X}^2_{p,t}] = \mathbf{a}_t^\top \boldsymbol{X}^1_{p,t}+\mathbf{b}_t^\top \mathbb{E}[\boldsymbol{X}^2_{p, t_\mathit{ref}}]+\eta^1_t
\]
\begin{multline*}
	\sigma_c^2 = \operatorname{Var}[\mathbf{a}_t^\top \boldsymbol{X}^1_{p,t}+\mathbf{b}_t^\top \boldsymbol{X}^2_{p, t_\mathit{ref}}+\eta^1_t|\boldsymbol{X}^1_{p,t},\boldsymbol{X}^2_{p,t}] \\
	= \operatorname{Var}[\mathbf{a}_t^\top \boldsymbol{X}^2_{p, t_\mathit{ref}}|\boldsymbol{X}^2_{p,t}] + \operatorname{Var}[\eta^1_t] = \mathbf{b}_t^\top \operatorname{Cov}[\boldsymbol{X}^2_{p, t_\mathit{ref}}] \mathbf{b}_t + \sigma_{1,t}
\end{multline*}
with $\operatorname{Cov}[\boldsymbol{X}^2_{p, t_\mathit{ref}}] = \mathbb{E}[(\boldsymbol{X}^2_{p, t_\mathit{ref}}-\mathbb{E}|\boldsymbol{X}^2_{p, t_\mathit{ref}}])(\boldsymbol{X}^2_{p, t_\mathit{ref}}-\mathbb{E}|\boldsymbol{X}^2_{p, t_\mathit{ref}}])^\top]$.

\begin{multline*}
	\mathbb{E}_{(\boldsymbol{X}^1_{p,t},\boldsymbol{X}^2_{p,t})}[(\mu_a-\mu_c)^2] = \mathbb{E}_{(\boldsymbol{X}^1_{p,t},\boldsymbol{X}^2_{p,t})}[(\mathbf{b}_t^\top (\boldsymbol{X}^2_{p,t} - \mathbb{E}[\boldsymbol{X}^2_{p, t_\mathit{ref}}]))^2] \\
	= \mathbf{b}_t^\top \mathbb{E}[(\boldsymbol{X}^2_{p,t}-\mathbb{E}|\boldsymbol{X}^2_{p, t_\mathit{ref}}])(\boldsymbol{X}^2_{p,t}-\mathbb{E}|\boldsymbol{X}^2_{p, t_\mathit{ref}}])^\top] \mathbf{b}_t
\end{multline*}

Therefore, the non-zero-mean Causal Strength with reference states is 
\begin{multline*}
	\text{rDCS}(X^2_t\rightarrow X^1_t) 
	= \frac{1}{2} \log \frac
	{\sigma_{1,t} + \mathbf{b}_t^\top \operatorname{Cov}[\boldsymbol{X}^2_{p, t_\mathit{ref}}] \mathbf{b}_t  }
	{\sigma_{1,t} } 
	- \frac{1}{2} \\
	+ \frac{1}{2} \cdot \frac
	{\sigma_{1,t} + \mathbf{b}_t^\top \mathbb{E}[(\boldsymbol{X}^2_{p,t}-\mathbb{E}[\boldsymbol{X}^2_{p, t_\mathit{ref}}])(\boldsymbol{X}^2_{p,t}-\mathbb{E}[\boldsymbol{X}^2_{p, t_\mathit{ref}}])^\top] \mathbf{b}_t}
	{\sigma_{1,t} + \mathbf{b}_t^\top \operatorname{Cov}[\boldsymbol{X}^2_{p, t_\mathit{ref}}] \mathbf{b}_t} 
\end{multline*}

Notably, when rDCS is applied to the models where we don't have explicit access of the \textit{i.i.d.} samples for ${\boldsymbol{X}_{p,t}^2}$, the term $\mathbb{E}[(\boldsymbol{X}^2_{p,t}-\mathbb{E}[\boldsymbol{X}^2_{p, t_\mathit{ref}}])(\boldsymbol{X}^2_{p,t}-\mathbb{E}[\boldsymbol{X}^2_{p, t_\mathit{ref}}])^\top]$ should be expanded as:
\begin{multline} \label{eq:rDCS_desnap}
	\mathbb{E}[(\boldsymbol{X}^2_{p,t}-\mathbb{E}[\boldsymbol{X}^2_{p, t_\mathit{ref}}])(\boldsymbol{X}^2_{p,t}-\mathbb{E}[\boldsymbol{X}^2_{p, t_\mathit{ref}}])^\top] \\
	= \mathbb{E}[\boldsymbol{X}^2_{p,t} {\boldsymbol{X}^2_{p,t}}^\top] 
	- \mathbb{E}[ \boldsymbol{X}^2_{p,t} \mathbb{E}[\boldsymbol{X}^2_{p, t_\mathit{ref}}]^\top]
	- \mathbb{E}[\mathbb{E}[\boldsymbol{X}^2_{p, t_\mathit{ref}}]^\top {\boldsymbol{X}^2_{p,t}}^\top]
	+ \mathbb{E}[\mathbb{E}[\boldsymbol{X}^2_{p, t_\mathit{ref}}]\mathbb{E}[\boldsymbol{X}^2_{p, t_\mathit{ref}}]^\top] \\
	=\operatorname{Cov}(\boldsymbol{X}^2_{p,t}) +\mathbb{E}[\boldsymbol{X}^2_{p,t}]\mathbb{E}[\boldsymbol{X}^2_{p,t}]^\top
	- \mathbb{E}[\boldsymbol{X}^2_{p,t}]\mathbb{E}[\boldsymbol{X}^2_{p,t_\mathit{ref}}]^\top \\
	- \mathbb{E}[\boldsymbol{X}^2_{p,t_\mathit{ref}}]\mathbb{E}[\boldsymbol{X}^2_{p,t}]^\top
	+ \mathbb{E}[\boldsymbol{X}^2_{p, t_\mathit{ref}}]\mathbb{E}[\boldsymbol{X}^2_{p, t_\mathit{ref}}]^\top
\end{multline}




\bibliographystyle{unsrtnat}
\bibliography{exported-references-multiTrialGranger}
\end{document}
